# Supplementary material for: Data-driven discovery of non-Newtonian astronomy via learning non-Euclidean Hamiltonian
Source: arXiv:2210.00090 source file (2022-09-30)
Supplement: Supplementary file 1 [file appendix.tex]

%!TEX root = ../main.tex

% \crefalias{section}{appendix}
% \crefalias{subsection}{appendix}

% Redefine section to reset equation number to 0.
\makeatletter
\let\origsection\section
\renewcommand\section{\@ifstar{\starsection}{\nostarsection}}

\newcommand\nostarsection[1]
{\sectionprelude\origsection{#1}\sectionpostlude}

\newcommand\starsection[1]
{\sectionprelude\origsection*{#1}\sectionpostlude}

\newcommand\sectionprelude{%
}

% Reset the equation number at the beginning of each section.
\newcommand\sectionpostlude{%
  \setcounter{equation}{0}
}
\makeatother

% % \renewcommand{\thesection}{SM-\arabic{section}} 

% Reference equations by the Appendix number + equation number. ex. (A.1).

% Undo all of the space saving stuff done for the main paper for better readability.
\makeatletter
% Spacing for Math.
\renewcommand{\normalsize}{%
  \@setfontsize\normalsize\@xpt\@xipt
  \abovedisplayskip      7\p@ \@plus 2\p@ \@minus 3\p@
  \abovedisplayshortskip \z@ \@plus 3\p@
  \belowdisplayskip      \abovedisplayskip
  \belowdisplayshortskip 4\p@ \@plus 3\p@ \@minus 3\p@
}
\normalsize

% paragraphs - Reset looseness.
\let\markeverypar\everypar
\newtoks\everypar
\everypar\markeverypar
\markeverypar{\the\everypar\looseness=0\relax}

% mathspacing
\thinmuskip=3.2mu plus 3mu
\medmuskip=4.2mu plus 2.0mu minus 4.0mu
\thickmuskip=5.2mu plus 5.0mu

\makeatother

%%%%%%%%%%%%%%%%%%%%%%%%%%%%%%%%%%%%%%%%%%%%%%%%%%%%%%%%%

\section{Rigid Body Equations of Motion} \label{app:rigid_body_eom}
We present two derivations from \citet{chen2021grit}. The first derivation derives a constrained Hamiltonian system via Lagrange multipliers, while the second uses a variational principle for mechanics on Lie groups. We also note that the same equations can be derived via the use of the Port-Hamiltonian framework as in \citet{duong2021hamiltonian}, though they choose to express the linear momentum coordinates in the moving body frame rather than the inertial frame as is done in this work.
%%%%%%%%%%%%%%%%%%%%%%%%%%%%%%%%%%%%%%%%%%%%%%%%%%%
\subsection{Constrained Hamiltonian System}
Since the manifold $\mathsf{SE}(3)^{\otimes N}$ is a product space of the individual manifolds $\mathsf{SE}(3)$, we consider the latter for brevity and drop indices $i$ for each body. Furthermore, $\mathsf{SE}(3)$ can be seen as the product space of $\Rb^3 \times \mathsf{SO}(3)$ for which the former is unconstrained, so we focus our attention on the latter.
We can view $\vR$ to be in the embedded Euclidean space $\vR^{3 \times 3} \xhookleftarrow{} \mathsf{SO}(3)$ and use $\vR \in \mathsf{SO}(3) \coloneqq h(\vR) = \{ \vR\T \vR - \vId = \vb{0}_{3\times3} \}$ as a holonomic constraint. Using Lagrange multipliers $\vLambda$ \cite{hairerGeometricNumericalIntegration2006} for the constraint $h$ gives us the following Lagrangian
\begin{equation} \label{eq:app:L}
    L(\vR, \dot{\vR}) = \frac{1}{2} \Tr\left[ \dot{\vR} \vJd{} \dot{\vR} \right] - V(\vR) - \frac{1}{2} \Tr\left[ \vLambda\T (\vR\T \vR - \vId )\right]
\end{equation}
where $\vJd{}$ denotes the nonstandard moment of inertia \cite{chen2021grit,taeyoungleeliegroup2005}
\begin{equation}
    \vJd \coloneqq \int_{\mathcal{B}} \rho(\vb{x}) \vb{x} \vb{x}\T \dd{\vb{x}}, \qquad
    \vJd = \Tr[ \vJ ] \vId - \vJ, \qquad
    \vJ = \Tr[\vJd] \vId - \vJd,
\end{equation}
and
\begin{equation}
    \vLambda = \begin{bmatrix}\lambda_1 & \lambda_4 & \lambda_6 \\ \lambda_4 & \lambda_2 & \lambda_5 \\ \lambda_6 & \lambda_5 & \lambda_3\end{bmatrix} \in \Rb^{3 \times 3}
\end{equation}
is a 6-dimensional symmetric matrix of Lagrange multipliers. Performing the Legendre transform for \eqref{eq:app:L} gives us the conjugate rotational momentum $\vP$ as
\begin{equation}
    \vP = \pdv{L(\vR, \dot{\vR})}{\dot{\vR}} = \dot{\vR} \vJd
\end{equation}
and corresponding Hamiltonian
\begin{equation}
    H(\vR, \vP)
    = \frac{1}{2}\Tr\left[\vP{} \vJd{}^{-1} \vP{}\right] + V(\vR)
    + \frac{1}{2}\Tr\left[\vLambda\T (\vR\T \vR - \vId)\right]
\end{equation}
The constraint for $\vP$ can be obtained by taking the time derivative of $h(\vR) = 0$ according to \citet{haier2006geometric}, i.e., $\vJd^{-1} \vP\T \vR + \vR\T \vP \vJd^{1} = \vb{0}_{3\times3}$. Hence, our equations of motion so far looks like 
\begin{equation}
    \begin{dcases}
        \dot{\vR} = \pdv{H}{\vP} = \vP \vJd^{-1} \\
        \dot{\vP} = -\pdv{H}{\vR} = -\pdv{V}{\vR} - \vR \vLambda
    \end{dcases}
\end{equation}
on the manifold
\begin{equation}
    \mathcal{M} \coloneqq \{ (\vR, \vP) | \vR\T \vR = \vId, \quad  \vJd^{-1} \vP\T \vR + \vR\T \vP \vJd^{-1} = \vb{0}_{3\times3}
\end{equation}
Let $\hat{\vOmega} = \vR\T \dot{\vR}$ denote the body's angular velocity in the inertial frame, where $\wedge$ denotes the cross-product operation $\hat{u} v = u \times v$. Then, it can written using $P$ as
\begin{equation}
    \hat{\vOmega} = \vR\T \vP \vJd^{-1}
\end{equation}
Taking the time derivative of $\hat{\vOmega}$ gives
\begin{equation}
    \dot{\hat{\vOmega}} = \vJd^{-1} \vP\T \vP \vJd^{-1} + \vR\T \left( -\pdv{V(\vR)}{\vR} - \vR \vLambda \right) \vJd^{-1}
\end{equation}
Since our goal is to represent the dynamics of $\vPi$, we convert the above to the body frame momentum using $\vPi = \vJ \vOmega$. Using properties of the hat map \cite[Appendix A.1]{chen2021grit} gives us
\begin{equation}
    \hat{\vPi}
    = \hat{\vJ \vOmega}
    = \Tr[\vJd] \hat{\vOmega} - \widehat{\vJd \vOmega}
    = \hat{\vOmega} \vJd{} - \vJd{} \hat{\vOmega}\T.
\end{equation}
Taking the time derivative of the above then gives
\begin{align}
    \dot{\hat{\vPi}}
    &= \dot{\hat{\vOmega}} \vJd{} - \vJd{} \dot{\hat{\vOmega}}, \\
    &= \left( \vJd^{-1} \vP\T \vP - \vP\T \vP \vJd^{-1} \right)
    -  \left( \vR\T\pdv{V(\vR)}{\vR} + \left( \pdv{V(\vR)}{\vR} \right)\T\vR \right)
    - \left( \vLambda - \vLambda\T \right), \\
    &= \left( \vJd^{-1} \vP\T \vP - \vP\T \vP \vJd^{-1} \right)
    -  \left( \vR\T\pdv{V(\vR)}{\vR} + \left( \pdv{V(\vR)}{\vR} \right)\T\vR \right),
\end{align}
where the symmetric $\vLambda$ vanishes on the last line.

Since $\vP = \vR \hat{\vOmega} \vJd{}$, applying properties of the hat map \cite[Appendix A.1]{chen2021grit} further simplifies the above as
\begin{align}
    \hat{\dot{\vPi}}
    &= \left( \hat{\vOmega}\T \hat{\vOmega} \vJd{} - \vJd{} \hat{\vOmega}\T \hat{\vOmega} \right)
    -  \left( \vR\T\pdv{V(\vR)}{\vR} + \left( \pdv{V(\vR)}{\vR} \right)\T\vR \right), \\
    &= \widehat{\vOmega \times \vJd{} \vOmega }
    -  \left( \vR\T\pdv{V(\vR)}{\vR} + \left( \pdv{V(\vR)}{\vR} \right)\T\vR \right).
\end{align}
Thus, applying the vee map and converting back to $\vJ$ and $\vPi$ gives
\begin{align}
    \dot{\vPi}
    &= \vOmega \times \vJd{} \vOmega - \left( \vR\T\pdv{V(\vR)}{\vR} + \left( \pdv{V(\vR)}{\vR} \right)\T\vR \right)^{\vee}, \\
    &= \vOmega \times ()\Tr[\vJ] - \vJ)\vOmega - \left( \vR\T\pdv{V(\vR)}{\vR} + \left( \pdv{V(\vR)}{\vR} \right)\T\vR \right)^{\vee}, \\
    &= -\vOmega \times \vJ \vOmega - \left( \vR\T\pdv{V(\vR)}{\vR} + \left( \pdv{V(\vR)}{\vR} \right)\T\vR \right)^{\vee}, \\
    &= \vPi \times \vJ^{-1} \vPi - \left( \vR\T\pdv{V(\vR)}{\vR} + \left( \pdv{V(\vR)}{\vR} \right)\T\vR \right)^{\vee}.
\end{align}
Hence, the rotational equations of motion on $\mathsf{SO}(3)$ are
\begin{equation}
    \begin{dcases}
    \dot{\vR} = \vR \widehat{\vJ^{1} \vPi}, \\
    \dot{\vPi} = \vPi \times \vJ^{-1} \vPi - \left( \vR\T \pdv{V(\vR)}{\vR} - \left( \pdv{V(\vR)}{\vR}\right)\T \vR \right)^{\vee}.
    \end{dcases}
\end{equation}

%%%%%%%%%%%%%%%%%%%%%%%%%%%%%%%%%%%%%%%%%%%%%%%%%%%
\subsection{Variational Principle for Mechanics on the Lie Group}
We can also apply the Euler-Lagrange equations for Hamilton's variational principle on a Lie group, a topic that has been well studied (e.g., \citet{marsden2013introduction,holm2009geometric}) \cite{chen2021grit}, and we summarize the results for the special case of rigid bodies from the expository part of \citet{taeyoungleeliegroup2005}.

Denote the infinitesimally varied rotation by $\vR_\epsilon = \vR \exp(\epsilon \hat{\veta})$, with $\epsilon \in \Rb$ and $\veta \in \Rb^3$, where $\exp(\cdot)$ is the exponential map from $\mathfrak{so}(3)$ to $\mathsf{SO}(3)$. The varied angular velocity $\hat{\vOmega}_\epsilon$ is
\begin{align}
    \hat{\vOmega}_\epsilon
    &= \vR_\epsilon\T \dot{\vR}_\epsilon
    = \exp(-\epsilon \hat{\veta}) \left( \dot{\vR} \exp(\epsilon \hat{\veta}) + \vR \exp(\epsilon \hat{\veta}) \epsilon \hat{\veta} \right), \\
    &= \exp(-\epsilon \hat{\veta}) \hat{\vOmega} \exp(-\epsilon \hat{\veta}) + \exp(-\epsilon \hat{\veta}) \hat{\dot{\veta}}, \\
    &= \hat{\vOmega} + \epsilon \left( \hat{\dot{\veta}} + \hat{\vOmega} \hat{\veta} - \hat{\veta} \hat{\vOmega} \right) + O(\epsilon^2).
\end{align}
Consider the action 
\begin{equation}
    S(\vOmega, \vR)
    = \int_{t_0}^{t_1} L(\vOmega, \vR) \dd{t}
    = \int_{t_0}^{t_1} \frac{1}{2} \Tr[ \hat{\vOmega} \vJd{} \hat{\vOmega} ] - V(\vR) \dd{t}.
\end{equation}
Taking the variation $S_\epsilon$ of the action $S$, we have
\begin{equation}
\begin{split}
    S_\epsilon(\vOmega, \vR)
    &= S(\vOmega_\epsilon, \vR_\epsilon), \\
    &= S(\vOmega, \vR)
        + \epsilon \int_{t_0}^{t_1} \bigg\{ \frac{1}{2} \Tr\Big[
            -\hat{\dot{\veta}} \left( \vJd{} \hat{\vOmega} + \hat{\vOmega} \vJd{} \right) \\
    &\quad + \hat{\veta} \hat{\vOmega} \left( \vJd{} \hat{\vOmega} + \hat{\vOmega} \vJd{} \right) - \hat{\veta} \left( \vJd{} \hat{\vOmega} + \hat{\vOmega} \vJd{} \hat{\vOmega} \right)
        \Big] + \Tr[ \hat{\veta} \vR\T \pdv{V(\vR)}{\vR}] \bigg\} \dd{t} \\
    &\quad+ O(\epsilon^2).
\end{split}
\end{equation}
Using \textit{Hamilton's Principle}, we have $\eval{\dv{\epsilon}}_{\epsilon=0} S_\epsilon = 0$, i.e.,
\begin{equation}
    \frac{1}{2} \int_{t_0}^{t_1} \Tr\left[ \hat{\veta} \left\{
            \widehat{\vJ \dot{\vOmega}} + \widehat{\vOmega \times \vJ \vOmega} + 2 \vR\T \pdv{V(\vR)}{\vR}
        \right\} \right] \dd{t} = 0,
\end{equation}
for any $\veta \in \Rb^3$. Hence, $\widehat{\vJ \dot{\vOmega}} + \widehat{\vOmega \times \vJ \vOmega} + 2 \vR\T \pdv{V(\vR)}{\vR}$ must be skew-symmetric, giving us
\begin{equation}
    \widehat{\vJ \dot{\vOmega}} = -\widehat{\vOmega \times \vJ \vOmega} + \left( \pdv{V(\vR)}{\vR}\T \vR - \vR\T \pdv{V(\vR)}{\vR} \right).
\end{equation}
Thus, by definition of $\vPi$ and applying the vee map, we recover the same update
\begin{equation}
    \dot{\vPi} = \vPi \times \vJ^{-1} \vPi + \left( \pdv{V(\vR)}{\vR}\T \vR - \vR\T \pdv{V(\vR)}{\vR} \right)^{\vee}.
\end{equation}
\section{Details of the \texorpdfstring{\LieT}{Lie T2} splitting integrator} \label{app:integrator_details}
The full Hamiltonian $H$ takes the form
\begin{equation}
    \Ham(\vq, \vR, \vp, \vPi) = \sum_{i=1}^N \frac{1}{2} \vp_i\T \vp_i / m_i + \frac{1}{2} \vPi_i\T \vJ_i^{-1} \vPi_i + V(\vq, \vR)
\end{equation}
We borrow from \citet{chen2021grit} the idea of Lie-group and symplecticity preserving splitting and split our Hamiltonian as
$\Ham = \mathcal{H}_{\KE} + \mathcal{H}_{\PE} + \mathcal{H}_{\asym}$, where
\begin{align}
    \mathcal{H}_{\KE} &\coloneqq \sum_{i=1}^N \frac{1}{2} \vp_i\T \vp_i / m_i + \frac{1}{2} \vPi_i\T \vJ_{i,\text{sym}}^{-1} \vPi_i \\
    \mathcal{H}_{\PE} &\coloneqq V(\vq, \vR) \\
    \mathcal{H}_{\asym} &\coloneqq \sum_{i=1}^N \frac{1}{2} \vPi_i\T \vJ_{i, \asym}^{-1} \vPi_i
\end{align}
where we assume that $\vJ_i$ is axis-symmetric, i.e.,
\begin{equation}
    \vJ_i \coloneqq \begin{bmatrix}
        J_i^{(1)} & 0 & 0 \\
        0 & J_i^{(2)} & 0 \\
        0 & 0 & J_i^{(3)}
    \end{bmatrix}
\end{equation}
and $\vJ_{i, \text{sym}}^{-1}$ and $\vJ_{i, \asym}^{-1}$ denote the axial-symmetric and residual terms of $\vJ_i^{-1}$ such that $\vJ_{i, \text{sym}}^{-1} + \vJ_{i, \asym}^{-1} = \vJ_i^{-1}$, i.e.,
\begin{equation}
    \vJ_{i,\text{sym}}^{-1} \coloneqq \begin{bmatrix}
        1 / J_i^{(1)} & 0 & 0 \\
        0 & 1 / J_i^{(1)} & 0 \\
        0 & 0 & 1 / J_i^{(3)}
    \end{bmatrix},
    \qquad
    \vJ_{i,\text{asym}}^{-1} \coloneqq \begin{bmatrix}
        0 & 0 & 0 \\
        0 & 1 / J_i^{(2)} - 1/J_i^{(1)} & 0 \\
        0 & 0 & 0
    \end{bmatrix}.
\end{equation}
Then, each of $\mathcal{H}_{\KE} + \mathcal{H}_{\PE} + \mathcal{H}_{\asym}$ can be integrated exactly.

\paragraph{Exact integration of $\bm{\mathcal{H}_{\KE}}$}
For $\mathcal{H}_{\KE}$, we have the equations of motion (using \eqref{eq:dyn:qdot}-\eqref{eq:dyn:Pidot} but with $V=0$)
\begin{subequations}
\begin{empheq}[left={\empheqlbrace}]{align}
    \dot{\vq}_i &= \vp_i / m_i \\
    \dot{\vp}_i &= 0 \\
    \dot{\vR}_i &= \vR{}_i \widehat{\vJ_{i, \text{sym}}^{-1} \vPi_i} \label{eq:app:ke_Rdot} \\
    \dot{\vPi}_i &= \vPi{}_i \times \vJ_{i, \text{sym}}^{-1} \vPi_i \label{eq:app:ke_pidot}
\end{empheq}
\end{subequations}
The equation for $\dot{\vPi}_i$ \eqref{eq:app:ke_pidot} is the Euler equation for a free rigid body \cite{chen2021grit}. It is exactly solvable with a simple expression for axial-symmetric bodies, since in this case $\dot{\vPi}$ simplifies as
\begin{equation}
    \dot{\vPi}_i
    = \vPi_{i} \times \vJ_{i, \sym}^{-1} \vPi_i
    = \begin{bmatrix}
        \left( 1 / J_i^{(3)} - 1 / J_i^{(1)} \right) \Pi_{i, y} \Pi_{i, z} \\
        - \left( 1 / J_i^{(3)} - 1 / J_i^{(1)} \right) \Pi_{i, y} \Pi_{i, z} \\
        0
    \end{bmatrix}
\end{equation}
Consequently, $\Pi_{i,z}(t) = \Pi_{i,z}(0)$, meaning that we can express the above as the linear differential equation
\begin{align}
    \dot{\vPi}_i(t)
    &=
    \begin{bmatrix}
        0 & \left( 1 / J_i^{(3)} - 1 / J_i^{(1)} \right) \Pi_{i, z}(0) & 0 \\
        -\left( 1 / J_i^{(3)} - 1 / J_i^{(1)} \right) \Pi_{i, z}(0) & 0 & 0 \\
        0 & 0 & 0
    \end{bmatrix}
    \vPi_i(0) \\
    &= -\theta t \widehat{\begin{bmatrix}0\\0\\1\end{bmatrix}} \vPi_i(0)
\end{align}
where $\theta \coloneqq \left(1 / J_i^{(3)} - 1 / J_i^{(1)}\right) \Pi_{i, z}(0)$ and has the solution
\begin{equation}
    \vPi_i(t) = \exp\left(-\theta t \widehat{\begin{bmatrix}0\\0\\1\end{bmatrix}} \right) \vPi_i(0) = R_z\T(\theta t) \vPi_i(0)
\end{equation}
where $R_z$ denotes the rotation matrix around the $z$ axis. Taking the above back to \eqref{eq:app:ke_Rdot} then gives us the solution for $\vR_i$ as well, giving the flow $\phi_h^{[\KE]}$ of $\Ham_{\KE}$ as
\begin{equation}
    \begin{dcases}
        \vq_i(h) = \vq_i(0) + \vp_i / m_i h, \\
        \vp_i(h) = \vp_i(0), \\
        \vR_i(h) = \vR_i(0) R_{\vPi_i(0)} \left( \norm{\vPi_i(0)} h / J_i^{(1)} \right) R_z(\theta h), \\
        \vPi_i(h) = R\T_z(\theta h) \vPi_i(0).
    \end{dcases}
\end{equation}

\paragraph{Exact integration of $\bm{\Ham_{\PE}}$}
For $\Ham_{\PE}$, the equations of motion are \cite{chen2021grit}
\begin{equation}
    \begin{dcases}
        \dot{\vq}_i = 0,
        \dot{\vp}_i = -\pdv{V}{\vq_i}, \\
        \dot{\vR}_i = 0,
        \dot{\vPi}_i = -\left( \vR_i\T \pdv{V}{\vR_i} - \left( \pdv{V}{\vR_i} \right)\T \vR_i \right)^\vee.
\end{dcases}
\end{equation}
Since $\vq_i$ and $\vp_i$ stay constant, $\vp_i$ and $\vPi_i$ change at constant rates. Hence, the flow $\phi_h^{[\PE]}$ of $\Ham_{\PE}$ is given by
\begin{equation}
    \begin{dcases}
        \vq_i(h) = \vq_i(0) \\
        \vp_i(h) = \vp_i(0) - \pdv{V}{\vq_i} h, \\
        \vR_i(h) = \vR_i(0), \\
        \vPi_i(h) = \vPi_i(0) - \left( \vR_i\T \pdv{V}{\vR_i} - \left( \pdv{V}{\vR_i} \right)\T \vR_i \right)^\vee h.
    \end{dcases}
\end{equation}

\paragraph{Exact integration of $\bm{\Ham_{\asym}}$}
Finally, the equations of motion of $\Ham_{\asym}$ are given by (again adapting \eqref{eq:dyn:qdot}-\eqref{eq:dyn:Pidot})
\begin{equation}
    \begin{dcases}
        \dot{\vq}_i = 0,
        \dot{\vp}_i = 0, \\
        \dot{\vR}_i = \vR_i \widehat{ \vJ_{i,\asym}^{-1} \vPi_i },
        \dot{\vPi}_i = \vPi_i \times \vJ_{i,\asym}^{-1} \vPi_i.
\end{dcases}
\end{equation}
which can be solved to obtain the flow $\phi_h^{[\asym]}$ of $\Ham_{\asym}$ as
\begin{equation}
    \begin{dcases}
        \vq_i(h) = \vq_i(0) \\
        \vp_i(h) = \vp_i(0), \\
        \vR_i(h) = R_y(\delta \Pi_i^{(2)} h) \vR_i(0), \\
        \vPi_i(h) = R_y(-\delta \Pi_i^{(2)} h) \vPi_i(0).
    \end{dcases}
\end{equation}
where $\delta \coloneqq 1 / J_i^{(2)} - 1 / J_{i}^{(1)}$.

Having obtained analytical solutions for each of the flows $\phi^{[\KE]}, \phi^{[\PE]}, \phi^{[\asym]}$, we then combine them with the non-conservative momentum update from the non-conservative forcing terms $F_{\vp_i}$ and $F_{\vPi_i}$ with flow $\phi_h^{[\force]}$
\begin{equation}
    \vq_i(h) = \vq_i(0) \\
    \vp_i(h) = \vp_i(0) + F_{\vp_i} h, \\
    \vR_i(h) = \vR_i(0), \\
    \vPi_i(h) =\vPi_i(0) + F_{\vPi_i} h.
\end{equation}
Consequently, the full \LieT{} integrator is obtained by applying the Strang composition scheme to obtain
\begin{equation}
    \phi_h^{\LieT} \coloneqq \phi_{h/2}^{[\KE]} \circ \phi_{h/2}^{[\PE]} \circ \phi_{h/2}^{[\asym]} \circ \phi_{h}^{[\force]} \circ \phi_{h/2}^{[\asym]} \circ \phi_{h/2}^{[\PE]} \circ \phi_{h/2}^{[\KE]}
\end{equation}
\section{Training Details} \label{app:training_details}
We implement our method using \texttt{Jax}\footnote{\href{https://github.com/google/jax}{https://github.com/google/jax}. The repository is licensed under Apache-2.0.} \cite{jax2018github} and use the \texttt{Haiku} framework \cite{haiku2020github}\footnote{\href{https://github.com/deepmind/dm-haiku}{https://github.com/deepmind/dm-haiku}. The repository is licensed under Apache-2.0.} for constructing the deep neural networks. In all our experiments, we use a multilayer perceptron (MLP) with $3$ hidden layers each of size $256$ with the SiLU activation \cite{elfwing2018sigmoid} for all networks ($V_{\text{resid}}^\theta, F^\theta_p, F^\theta_\Pi$). Each method is run until convergence.
Other common training hyperparameters used are summarized in \cref{app:train_hyperparams}.

\paragraph{Structure of $V_{\textrm{resid}}^\theta$}
Note that we \textbf{do not} assume prior knowledge on the pairwise structure of the potential function $V_{\text{resid}}$ or of the forcing terms $F_{\bf{p}}, F_{\bf{\Pi}}$.
More specifically, since the true Gravitational potential \eqref{eq:grav_potential} only acts \textit{pairwise} between rigid bodies, the rigid body correction potential also acts pairwise and has the structure
\begin{equation}
    V_{\text{resid}}(\vq, \vR) = \sum_{i < j} V_{i, j, \text{resid}}(\vq_i, \vq_j, \vR_i, \vR_j).
\end{equation}
For the forcing terms, the tidal forcing term also acts pairwise with coupled effects on $\bf{\vp}_i$ and $\bf{\Pi}_i$ due the relationship between forces and torques, while the post-Newton general-relativity correction term acts on each planet individually and affects only $\bf{\vp}_i$. However, in this work, we assume that none of this prior knowledge is available and aim to learn everything purely from data. Hence, we choose to learn the high dimensional forms of $V_{\text{resid}}, F_{\bf{p}}, F_{\bf{\Pi}}$.
The fact that we were able to obtain improvements despite the high dimensionality of the input space ($8$ planets each with $(\vq_i, \vR_i) \in \Rb^{3} \times \Rb^{3 \times 3} \approx \Rb^{12}$, i.e., $\Rb^{96}$ for $V$ and $\Rb^{144}$ for $F_{\bf{p}}, F_{\bf{\Pi}}$) is an indication of the generality of our approach. We believe that the proposed approach can be made more scalable and have better generalization if we do assume some knowledge about the structure of the forces at play and instead, e.g., learn $V_{\text{resid}}^\theta(\vq_i, \vq_j, \vR_i, \vR_j, \phi_i, \phi_j)$ instead of the more general $V_{\text{resid}}^\theta(\vq, \vR)$ and similarly for the forcing terms, where $\phi_i, \phi_j$ contains known or potentially learned information about physical properties about each rigid body which are needed. Here, since the ordering of $i$ and $j$ is not important, some type of permutation-invariant encoding such as \cite{lee2019set} should be used to further improve generalization.

\paragraph{Training} All experiments are done on a single RTX 3090 locally. The length of each run is dependent on the complexity of the integrator. For example, explicit Euler is the simplest and has the fastest per-iteration time, while Lie RK4 has the slowest per-iteration time. The Lie T2 integrator has a per-iteration time between the two extremes with each experiment taking approximately three hours.

\begin{table}
    \centering
    \caption{Common hyperparameters used for training in all experiments.}
    \bigskip
    \label{app:train_hyperparams}
    \begin{tabular}{ll}
        \toprule
        Name  & Value \\
        \midrule
        Batch size & $256$ \\
        Optimizer & \texttt{AdamW} \cite{loshchilov2017decoupled} \\
        Learning Rate & \num{4e-4} \\
        \bottomrule
    \end{tabular}
\end{table}

\paragraph{Data generation} We use the GRIT\footnote{\href{https://github.com/GRIT-RBSim/GRIT}{https://github.com/GRIT-RBSim/GRIT}. The repository is licensed under Apache-2.0.} simulator \cite{chen2021grit} for generating the dataset in all cases. Each dataset consists of \num{32} different trajectories, which is then split in a $80$-$20$ training-validation split. Each trajectory is then further subsampled to provide $128$ tuples $(\vq, \vR, \vp, \vPi)$ of datapoints. Each trajectory is generated by adding small multiplicative Gaussian noise to the coordinates of each body.

\subsection{Toy Two-Body Problem}
The parameters for this system were hand-picked to provide intuition on how the additional corrections differ from the pure point-mass potential that is widely used in other Hamiltonian learning literature.

\subsection{TRAPPIST-1}
The initial conditions for this system were taken directly from the TRAPPIST-1 example from GRIT.

\section{Details on Integrators used for Comparison in \cref{sec:results}}
\label{app:train_integrator_details}
To answer the question $\textbf{Q2}$ of how important are \textcolor{MaterialRedA200}{symplecticity} ($\SymSymbol$) and \textcolor{MaterialBlueA200}{Lie-group preservation} ($\LieSymbol$) for learning, we vary the choice of integrator in our experiments. The integrators used can be broadly split into four categories:

\noindent\textbf{Neither \textcolor{MaterialRedA200}{Symplectic} $\SymSymbol$ nor \textcolor{MaterialBlueA200}{Lie-group preserving} $\LieSymbol$: } This category contains the popular explicit Euler and Runge-Kutta 4 integrators, neither of which are symplectic or Lie-group preserving. The finite-difference scheme from \citet{greydanus2019hamiltonian,greydanus2022dissipative} can be interpreted as an application of the explicit Euler integrator \citet{david2021symplectic}. Explicit Euler is also used in the works of \citet{}. Runge-Kutta 4 is a popular fourth-order integrator due to its implementation simplicity and is used in \citet{finzi2020simplifying,zhongSymplecticODENetLearning2020,zhong2021benchmarking,zhong2021extending,duong2021hamiltonian}.

\noindent\textbf{\textcolor{MaterialRedA200}{Symplectic} $\SymSymbol$ but not \textcolor{MaterialBlueA200}{Lie-group preserving} $\LieSymbol$: } This category contains the verlet integrator, which we define loosely in the current work as the integrator obtained by using classical splitting and Strang composition, but \textit{without} performing exact integration on the manifold. In the Euclidean case where $\Ham(\vq, \vp) = \frac{1}{2} \vp\T \vp / m + V(\vq)$, this takes the form
\begin{align}
    \vq(h / 2) &= \vq(0) + \frac{\vp(0)}{m} h, \\
    \vp(h) &= \vp(0) - \pdv{V}{\vq} h, \\
    \vq(h) &= \vq(h / 2) + \frac{\vp(1)}{m} h, 
\end{align}
and corresponds to the ``leapfrog'' proposed in SRNN \citet{chen2019symplectic}.
In our setting where the space is not Euclidean, we interpret a ``naive'' implementation to look like the following
\begin{subequations}
\begin{empheq}[left={\empheqlbrace}]{align}
    \vq_i(h/2) &= \vq_i(0) + \frac{\vp_i(0)}{m} h, \\
    \vR_i(h/2) &= \vR_i(0) + \vb{R}_i(0) \; \widehat{\vb{J}_i^{-1} \vb{\Pi}_i(0)} h,
\end{empheq}%
\end{subequations}
\begin{subequations}
\begin{empheq}[left={\empheqlbrace}]{align}
    \vp_i(h) &= \vp_i(0) - \pdv{V}{\vq_i} h, \\
    \vPi_i(h) &= \vPi_i(0) + \left( \vPi_i(0) \times \vJ_i^{-1} \vPi_i(0) - \left(\vR_i\T(0) \pdv{V}{\vR_i} - \left(\pdv{V}{\vR_i}\right)\T \vR_i(0)\right)^\vee \right) h,
\end{empheq}
\end{subequations}
\begin{subequations}
\begin{empheq}[left={\empheqlbrace}]{align}
    \vq_i(h) &= \vq_i(h/2) + \frac{\vp_i(h)}{m} h, \\
    \vR_i(h) &= \vR_i(h/2) + \vb{R}_i(h) \widehat{\vb{J}_i^{-1} \vb{\Pi}_i(h)} h,
\end{empheq}
\end{subequations}

\noindent\textbf{Not \textcolor{MaterialRedA200}{Symplectic} $\SymSymbol$ but is \textcolor{MaterialBlueA200}{Lie-group preserving} $\LieSymbol$: } This category contains the Lie RK2 (CF2) and Lie RK4 (CF4) commutator-free Lie-group preserving integrators from \citet{celledoniCommutatorfreeLieGroup2003}. These integrators are Lie-group preserving but are not symplectic. Specifically, the flow of Lie RK2 is described by 
\begin{align}
\begin{dcases}
    \begin{bmatrix} \vq_i(h/2) \\ \vp_i(h/2) \\ \vPi_i(h/2) \end{bmatrix}
    &=
    \begin{bmatrix} \vq_i(0) \\ \vp_i(0) \\ \vPi_i(0) \end{bmatrix}
    +
    \begin{bmatrix} \dot{\vq}_i(0) \\ \dot{\vp}_i(0) \\ \dot{\vPi}_i(0) \end{bmatrix}
    h, \\
    F_1 &= \widehat{\vJ_i^{-1} \vPi_i(0)}, \\
    \vR_i(h/2) &= \exp( F_1 h/2 ) \vR_i(0),
\end{dcases} \\
\begin{dcases}
    \begin{bmatrix} \vq_i(h) \\ \vp_i(h) \\ \vPi_i(h) \end{bmatrix}
    &=
    \begin{bmatrix} \vq_i(0) \\ \vp_i(0) \\ \vPi_i(0) \end{bmatrix}
    +
    \begin{bmatrix} \dot{\vq}_i(h/2) \\ \dot{\vp}_i(h/2) \\ \dot{\vPi}_i(h/2) \end{bmatrix}
    h, \\
    F_2 &= \widehat{\vJ_i^{-1} \vPi_i(h/2)}, \\
    \vR_i(h) &= \exp( F_2 h ) \vR_i(0).
\end{dcases}
\end{align}
For Lie RK4, the coordinates in Euclidean space (i.e., $\vq, \vp, \vPi$) follow the normal RK4 integration in a similar fashion as above, while the flow of the $\vR$ coordinate is described by
\begin{align}
&\begin{dcases}
    F_1 = \widehat{\vJ_i^{-1} \vPi_i(0)}, \\
    \vR_i^1 = \exp( F_1 h/2 ) \vR_i(0),
\end{dcases} \\
&\begin{dcases}
    F_2 = \widehat{\vJ_i^{-1} \vPi_i^1}, \\
    \vR_i^2 = \exp( F_2 h/2 ) \vR_i(0),
\end{dcases} \\
&\begin{dcases}
    F_3 = \widehat{\vJ_i^{-1} \vPi_i^2}, \\
    \vR_i^3 = \exp( (F_3 - F_1 /2) h ) \vR_i^2,
\end{dcases} \\
&\begin{dcases}
    F_4 = \widehat{\vJ_i^{-1} \vPi_i^3}, \\
    \vR_i(h/2) = \exp\left(\frac{h}{12}(3F_1 + 2 F_2 + 2 F_3 - F_4 ) \right) \vR_i(0), \\
    \vR_i(h) = \exp\left(\frac{h}{12}(-F_1 + 2 F_2 + 2 F_3 + 3F_4 ) \right) \vR_i(h/2),
\end{dcases}
\end{align}
where the superscripts denote the intermediate outputs of each stage.

\noindent\textbf{Both \textcolor{MaterialRedA200}{Symplectic} $\SymSymbol$ and \textcolor{MaterialBlueA200}{Lie-group preserving} $\LieSymbol$: } This category contains our proposed \LieT{} integrator which is both symplectic and Lie-group preserving using a splitting technique that allows for exact integration, borrowed from \citet{chen2021grit}. See \cref{app:integrator_details} for a detailed derivation.
\section{Definition of Evaluation Metrics}
\label{app:eval_metrics}
% The errors $\norm{ \Delta \vq }_2$, $\norm{ \Delta \vR }$, $\norm{ \Delta \vp }_2$, $\norm{ \Delta \vPi }_2$
The errors $\norm{ \Delta \vq }_2$, $\norm{ \Delta \vR }$
in \cref{tab:trappist} and \cref{tab:trappist_easy} are computed by predicting a trajectory with $500$ integrator steps, and then computing
\begin{align}
    \Delta \vq_{k, l} &\coloneqq \vq_{k, l} - \hat{q}_{k, l}, \\
    \Delta \vR_{k, l} &\coloneqq \vR_{k, l} - \hat{R}_{k, l},
    % \Delta \vp_{k, l} &\coloneqq \vp_{k, l} - \hat{p}_{k, l}, \\
    % \Delta \vPi_{k, l} &\coloneqq \vPi_{k, l} - \hat{\Pi}_{k, l},
\end{align}
and the norm for $\vR \in \mathsf{SO}(3)^{\otimes N}$ is the geodesic computed as
\begin{equation}
    \norm{\vR} \coloneqq \sum_{i=1}^N \norm{\vR_i},
    \qquad
    \norm{\vR_i} \coloneqq \cos^{-1}\left( \frac{\tr(\vR_i\T \vR_i) -1}{2} \right)
\end{equation}
The numbers shown in the table are taken to be the mean across all $L K$ samples.

The errors $\norm{\Delta \dot{p}}$ and $\norm{\Delta \dot{\Pi}}$ in \cref{tab:trappist} are intended to measure how well the forces (both conservative and non-conservative) are learned. Consequently, these are computed along the dataset and not the predicted trajectory and are defined as
\begin{align}
    \Delta \dot{p}_k &= \frac{\hat{p}((k+1)h) - p(kh)}{h} - \frac{p((k+1)h) - p(kh)}{h}, \\
    \Delta \dot{\Pi}_k &= \frac{ \hat{\Pi}((k+1)h) - \Pi(kh) }{h} - \frac{ \Pi((k+1)h) - \Pi(kh) }{h},
\end{align}
where $\hat{p}$ and $\hat{\Pi}$ in the equation above denote the one-step predictions using the learned integrator $\phi_h$, \ie
\begin{equation}
    \hat{q}(h), \hat{p}(h), \hat{R}(h), \hat{\Pi}(h),
    \coloneqq \phi_h\big( q(0), p(0), R(0), \Pi(0) \big).
\end{equation}
Similarly, the errors $\norm{\Delta \pdv{V}{q}}_2$ and $\norm{\Delta \pdv{V}{q}}_2$ in \cref{tab:trappist_easy} measure how well the potential (and hence the conservative forces) have been learned. Hence, these are again computed along the dataset and not the predicted trajectory and are defined as
\begin{align}
    \norm{ \Delta \pdv{V}{\vq} }^2_2 &\coloneqq
        \norm{ \pdv{V^\theta_{\resid}}{\vq} - \pdv{V_{\resid}}{\vq} }^2_2, \\
    \norm{ \Delta \pdv{V}{\vR} }^2_2 &\coloneqq
        \sum_{i=1}^{N} \norm{
            \left( \vR_i\T\pdv{V^\theta_{\resid}}{\vR_i} - \left(\pdv{V^\theta_{\resid}}{\vR_i}\right)\T \vR_i \right)^\vee -
            \left( \vR_i\T\pdv{V_{\resid}}{\vR_i} - \left(\pdv{V_{\resid}}{\vR_i}\right)\T \vR_i \right)^\vee }^2_2,
\end{align}
where the additional manipulations for $\Delta \pdv{V}{\vR}$ denote the projection of $\vR_i\T \pdv{V}{\vR_i}$ on the skew-symmetric matrices. This is done because only the skew-symmetric part of $\vR_i\T \pdv{V}{\vR_i}$ is used in the equations of motion \eqref{eq:dyn:qdot}--\eqref{eq:dyn:Pidot} and hence the learned symmetric part can be arbitrarily defined.
\section{Limitations and Future Directions}
\label{app:limitations}
One big assumption we make in our work is that the masses and inertial tensors $m_i, \vJ_i$ are known. This may be a restricting assumption when applying this method to learning physics for rigid bodies where this information is not available and must be learned jointly with the physics, an approach taken in many works on learning with Hamiltonian structure (e.g., \cite{zhong2021benchmarking,duong2021hamiltonian}). Moreover, as discussed in \cref{app:training_details}, our framework does not assume that prior knowledge on the structure (e.g., pairwise, independent) of the potential or forcing terms is known. If we make this assumption, then additional physical properties for each rigid body may need to be provided to fully specify the structured physics (e.g., time lag and tide constants for tidal forcing).
Extending this framework to handle the learning of per-body physical properties at the same time is left for future work.

Another direction that we have not been able to explore in this work is the robustness of our method to noise in the dataset. In this work, we use a dataset generated using the GRIT \cite{chen2021grit} simulator (see \cref{app:training_details}). Consequently, the dataset used is clean and not corrupted by any noise. As noted in SRNN \citet{chen2019symplectic}, integrating for multiple consecutive timesteps may allow the network to better discern the true noiseless trajectory when computing the loss function. Moreover, the benefit from performing this multi-step training is integrator dependent, with improvements not observed when using the naive explicit Euler integration. Given that, 1. our configuration space now lies on a Lie-group manifold, and 2. the physics of our system are mutiscale,
exploring whether those insights are applicable to the problem considered in this work is a future interesting direction that will help inform practitioners wishing to apply this methodology to real world data.
% \input{subtex/10_app_proofs.tex}

% %%%%%%%%%%%%%%%%%%%%%%%%%%%%%%%%%%%%%%%%%%%%%%%%%%%%%%%%%
% \newpage
% \section{Scratch}
% \input{subtex/10_app_scratch.tex}
